# Supplementary material for: NoiseAttack: An Evasive Sample-Specific Multi-Targeted Backdoor Attack Through White Gaussian Noise
Source: arXiv:2409.02251 source file (2024-09-03)
Supplement: Supplementary file 1 [file Appendix.tex]

\appendix \label{sec:appendix}
